# Supplementary material for: EMG-GPT: Predictive Pretraining on Residual-Quantized EMG Tokens for Hand Pose Estimation
Source: arXiv:2610.05235 source file (2026-10-04)
Supplement: Supplementary file 1 [file tab_appendix_architecture_ablation.tex]

\begin{table}[h!]
\centering
\scriptsize
\setlength{\tabcolsep}{2.5pt}
\caption{Matched $K=1$, 20k-step validation architecture screen (seed 123). Frozen linear-probe pose MAE is the selection metric; token CE and held-out-user stage classification are diagnostics. $\Delta$shuffle is shuffled-history minus unshuffled token CE in bits/code, so positive values indicate temporal-context use.}
\label{tab:appendix-architecture-ablation}
\begin{tabular}{@{}llllrrrr@{}}
\toprule
Family & Frame input & Head & Params (M) & CE (bits/code) & $\Delta$shuffle & Linear-probe MAE ($^\circ$) & Stage BA/F1 \\
\midrule
Factorized & learned IDs & factorized & 44.8 & 12.04 & 1.45 & 16.00 & 0.62/0.61 \\
Codebook-conditioned & learned IDs & codebook & 44.5 & 12.15 & 1.30 & 16.20 & 0.59/0.59 \\
Codebook-conditioned & frozen RVQ sum & codebook & 40.4 & 12.13 & 1.31 & 16.05 & 0.60/0.59 \\
Spatial autoregressive & learned IDs & spatial AR & 42.6 & 8.65 & 0.98 & 16.27 & 0.48/0.46 \\
\addlinespace[2pt]
Tokenizer-only control & frozen RVQ sum & -- & -- & -- & -- & 17.26 & -- \\
\bottomrule
\end{tabular}
\end{table}
