# Supplementary material for: EMG-GPT: Predictive Pretraining on Residual-Quantized EMG Tokens for Hand Pose Estimation
Source: arXiv:2610.05235 source file (2026-10-04)
Supplement: Supplementary file 2 [file tab_appendix_architecture_design.tex]

\begin{table}[h!]
\centering
\scriptsize
\setlength{\tabcolsep}{3pt}
\caption{Candidate designs. All variants first encode each structured EMG frame and then use a causal temporal backbone. The table isolates the frame input and target-conditioning choices that differ.}
\label{tab:appendix-architecture-design}
\begin{tabular}{@{}p{0.16\linewidth}p{0.19\linewidth}p{0.29\linewidth}p{0.27\linewidth}@{}}
\toprule
Candidate & Frame input & Target conditioning & Output scoring / purpose \\
\midrule
Factorized & Learned code-index embeddings & Bidirectional same-frame decoder; all target positions predicted in parallel & Learned categorical vocabulary; tests a direct discrete-token baseline \\
Codebook--IDs & Learned code-index embeddings & Parallel channel--branch queries; no realized coarser target depth & Scaled cosine similarity to the matching frozen codebook \\
Codebook--RVQ sum & Sum of frozen RVQ vectors per channel--branch & Parallel channel--branch queries; position count remains $CB$ as $K$ grows & Tests tokenizer geometry at both input and output \\
Spatial AR & Learned code-index embeddings & Causal scan over target channel--branch positions using earlier realized same-frame codes & Learned categorical vocabulary; tests within-frame spatial dependence \\
RVQ sum + depth AR & Sum of frozen RVQ vectors per channel--branch & Finer target depths condition on realized coarser-depth reconstructions & Frozen-codebook scoring; selected hierarchical family for $K>1$ \\
\bottomrule
\end{tabular}
\end{table}
