# Supplementary material for: EMG-GPT: Predictive Pretraining on Residual-Quantized EMG Tokens for Hand Pose Estimation
Source: arXiv:2610.05235 source file (2026-10-04)
Supplement: Supplementary file 3 [file tab_appendix_capacity_controls.tex]

\begin{table}[h!]
\centering
\small
\caption{Capacity and backbone controls for the $K=1$ factorized family (validation, seed 123, 20k-step pretraining). Random denotes a randomly initialized backbone with the same frozen linear probe.}
\label{tab:appendix-capacity-controls}
\begin{tabular}{@{}lrrrr@{}}
\toprule
Backbone & Params (M) & Token CE (bits/code) & Pretrained MAE ($^\circ$) & Random MAE ($^\circ$) \\
\midrule
Compact & 10.71 & 12.07 & 16.32 & 17.89 \\
Base & 44.75 & 12.04 & 16.00 & 17.89 \\
Wide & 97.40 & 12.07 & 16.05 & 18.01 \\
Axial & 46.86 & 12.01 & 16.18 & 17.92 \\
\bottomrule
\end{tabular}
\end{table}
