# Supplementary material for: EMG-GPT: Predictive Pretraining on Residual-Quantized EMG Tokens for Hand Pose Estimation
Source: arXiv:2610.05235 source file (2026-10-04)
Supplement: Supplementary file 4 [file tab_appendix_final_condition_micro.tex]

\begin{table}[h!]
\centering
\scriptsize
\caption{Secondary test metrics micro-averaged within each generalization condition. These values retain User, Stage, and User+Stage separation but do not estimate variability across users.}
\label{tab:appendix-final-condition-micro}
\begin{tabular}{@{}llrrrr@{}}
\toprule
Task & Condition & MAE ($^\circ$) & RMSE ($^\circ$) & Landmark (mm) & Fingertip (mm) \\
\midrule
Regression & User & 12.74 & 18.06 & 16.22 & 26.70 \\
Regression & Stage & 16.25 & 22.85 & 21.95 & 37.29 \\
Regression & User, Stage & 16.59 & 23.31 & 22.63 & 38.66 \\
Tracking & User & 8.79 & 14.01 & 11.46 & 18.70 \\
Tracking & Stage & 12.37 & 18.22 & 16.80 & 28.34 \\
Tracking & User, Stage & 12.13 & 17.98 & 16.91 & 28.56 \\
\bottomrule
\end{tabular}
\end{table}
