# Supplementary material for: EMG-GPT: Predictive Pretraining on Residual-Quantized EMG Tokens for Hand Pose Estimation
Source: arXiv:2610.05235 source file (2026-10-04)
Supplement: Supplementary file 5 [file tab_appendix_final_configuration.tex]

\begin{table}[h!]
\centering
\small
\caption{Validation-locked final configurations. Regression and Tracking select checkpoints independently. Tracking uses the jointly evaluated full-adaptation, $\lambda_{\mathrm{vel}}=4$ configuration.}
\label{tab:appendix-final-config}
\begin{tabular}{@{}llrrrr@{}}
\toprule
Task & GPT step & Adaptation & $\lambda_{\mathrm{vel}}$ & Pose step & Val. MAE ($^\circ$) \\
\midrule
Regression & 280k & Full & 0 & 2,000 & 13.693 \\
Tracking & 400k & Full & 4 & 5,000 & 9.601 \\
\bottomrule
\end{tabular}
\end{table}
