# Supplementary material for: EMG-GPT: Predictive Pretraining on Residual-Quantized EMG Tokens for Hand Pose Estimation
Source: arXiv:2610.05235 source file (2026-10-04)
Supplement: Supplementary file 6 [file tab_appendix_final_protocol.tex]

\begin{table}[h!]
\centering
\scriptsize
\setlength{\tabcolsep}{3.5pt}
\caption{Locked token-adapted pose protocols. Duration columns give input/scored/stride seconds; steps give GPT/selected pose checkpoints. Tip denotes fingertip distance.}
\label{tab:appendix-final-protocol}
\begin{tabular}{@{}llclll@{}}
\toprule
Task & 25-to-50-Hz alignment & Duration (s) & Boundary pose & Selected loss & Steps \\
\midrule
Regression & linear & 6/5/6 & None & L1 + 0.01 tip & 280k/2,000 \\
Tracking & causal & 6/5/5 & GT at 1.04 s & L1 + 0.01 tip + 4 velocity & 400k/5,000 \\
\bottomrule
\end{tabular}
\end{table}
