# Supplementary material for: EMG-GPT: Predictive Pretraining on Residual-Quantized EMG Tokens for Hand Pose Estimation
Source: arXiv:2610.05235 source file (2026-10-04)
Supplement: Supplementary file 7 [file tab_appendix_final_regression_test.tex]

\begin{table}[h!]
\centering
\scriptsize
\caption{Locked Regression test results for EMG-GPT. Values are exact equal-user mean $\pm$ sample SD within each generalization condition.}
\label{tab:appendix-final-regression-test}
\begin{tabular}{@{}lrrrr@{}}
\toprule
Condition & MAE ($^\circ$) & RMSE ($^\circ$) & Landmark (mm) & Fingertip (mm) \\
\midrule
User ($n=20$) & 12.80 $\pm$ 1.08 & 18.10 $\pm$ 1.34 & 16.30 $\pm$ 1.29 & 26.83 $\pm$ 2.12 \\
Stage ($n=158$) & 16.30 $\pm$ 1.57 & 22.83 $\pm$ 2.07 & 22.02 $\pm$ 1.92 & 37.42 $\pm$ 3.36 \\
User, Stage ($n=20$) & 16.64 $\pm$ 1.30 & 23.33 $\pm$ 1.65 & 22.70 $\pm$ 1.39 & 38.78 $\pm$ 2.39 \\
\bottomrule
\end{tabular}
\end{table}
