# Supplementary material for: EMG-GPT: Predictive Pretraining on Residual-Quantized EMG Tokens for Hand Pose Estimation
Source: arXiv:2610.05235 source file (2026-10-04)
Supplement: Supplementary file 8 [file tab_appendix_final_runtime.tex]

\begin{table}[h!]
\centering
\small
\caption{Descriptive training time for the locked seed-123 models. Values sum authoritative Slurm allocation elapsed times for single-GPU jobs.}
\label{tab:appendix-final-runtime}
\begin{tabular}{@{}lrrr@{}}
\toprule
Task & GPT step & \shortstack{Cumulative pretraining\\GPU allocation (h)} & \shortstack{Cumulative downstream\\GPU allocation (h)} \\
\midrule
Regression & 280k & 87.7 & 26.7 \\
Tracking & 400k & 125.3 & 64.0 \\
\bottomrule
\end{tabular}
\end{table}
