# Supplementary material for: EMG-GPT: Predictive Pretraining on Residual-Quantized EMG Tokens for Hand Pose Estimation
Source: arXiv:2610.05235 source file (2026-10-04)
Supplement: Supplementary file 9 [file tab_appendix_final_secondary.tex]

\begin{table}[h!]
\centering
\scriptsize
\caption{Secondary test diagnostics. Metrics are micro-averaged over valid values; speed reports prediction/target in degrees per second. Recording-level bootstrap 95\% CIs for MAE are $[15.024,15.206]$ for Regression and $[11.088,11.266]$ for Tracking (2,000 resamples).}
\label{tab:appendix-final-secondary}
\begin{tabular}{@{}lrrrrr@{}}
\toprule
Task & MAE ($^\circ$) & RMSE ($^\circ$) & Landmark & Fingertip & Speed \\
\midrule
Regression & 15.065 & 21.361 & 20.028 & 33.747 & 36.5/70.5 \\
Tracking & 11.138 & 16.888 & 14.992 & 25.080 & 27.6/68.7 \\
\bottomrule
\end{tabular}
\end{table}
