# Supplementary material for: EMG-GPT: Predictive Pretraining on Residual-Quantized EMG Tokens for Hand Pose Estimation
Source: arXiv:2610.05235 source file (2026-10-04)
Supplement: Supplementary file 10 [file tab_appendix_final_tracking_test.tex]

\begin{table}[h!]
\centering
\scriptsize
\caption{Locked Tracking test results for EMG-GPT. Values are exact equal-user mean $\pm$ sample SD within each generalization condition.}
\label{tab:appendix-final-tracking-test}
\begin{tabular}{@{}lrrrr@{}}
\toprule
Condition & MAE ($^\circ$) & RMSE ($^\circ$) & Landmark (mm) & Fingertip (mm) \\
\midrule
User ($n=20$) & 8.89 $\pm$ 0.93 & 14.08 $\pm$ 1.29 & 11.59 $\pm$ 1.24 & 18.93 $\pm$ 2.16 \\
Stage ($n=158$) & 12.42 $\pm$ 1.43 & 18.18 $\pm$ 1.91 & 16.88 $\pm$ 1.80 & 28.46 $\pm$ 3.09 \\
User, Stage ($n=20$) & 12.18 $\pm$ 1.25 & 17.98 $\pm$ 1.63 & 16.93 $\pm$ 1.36 & 28.61 $\pm$ 2.46 \\
\bottomrule
\end{tabular}
\end{table}
