# Supplementary material for: EMG-GPT: Predictive Pretraining on Residual-Quantized EMG Tokens for Hand Pose Estimation
Source: arXiv:2610.05235 source file (2026-10-04)
Supplement: Supplementary file 11 [file tab_appendix_loss_ablation.tex]

\begin{table}[h!]
\centering
\small
\caption{Matched $K=4$ continuations from the same 230k checkpoint, each trained for 20k additional steps (validation, seed 123). }
\label{tab:appendix-loss-ablation}
\begin{tabular}{@{}lrrr@{}}
\toprule
Objective & Regression MAE ($^\circ$) & User+Stage MAE ($^\circ$) & Landmark (mm) \\
\midrule
Uniform hard CE & 14.59 & 17.87 & 19.27 \\
Inverse-depth CE & 14.51 & 17.82 & 19.14 \\
CE + latent & 14.95 & 18.29 & 19.99 \\
\bottomrule
\end{tabular}
\end{table}
