# Supplementary material for: EMG-GPT: Predictive Pretraining on Residual-Quantized EMG Tokens for Hand Pose Estimation
Source: arXiv:2610.05235 source file (2026-10-04)
Supplement: Supplementary file 12 [file tab_appendix_matched_adaptation.tex]

\begin{table}[h!]
\centering
\small
\caption{Matched downstream adaptation at $K=4$ and 25~Hz. Regression and Tracking select their source GPT independently from the 40k--400k validation sweep (280k and 400k, respectively). Within each task, the target index, decoder architecture, optimization budget, and seed are fixed; only the trainable portion of the GPT changes. Values are independent full-validation evaluations of the best downstream checkpoint.}
\label{tab:appendix-matched-adaptation}
\begin{tabular}{@{}llrrrr@{}}
\toprule
Task & GPT update & GPT step & Head step & MAE ($^\circ$) & User+Stage ($^\circ$) \\
\midrule
Regression & Frozen & 280k & 1,500 & 14.096 & 17.685 \\
Regression & Top-2 & 280k & 2,000 & 14.056 & 17.608 \\
Regression & Full & 280k & 2,000 & \textbf{13.693} & 17.086 \\
\hline
\addlinespace[2pt]
Tracking & Frozen & 400k & 5,000 & 9.758 & 13.126 \\
Tracking & Top-2 & 400k & 1,500 & 9.749 & 13.087 \\
Tracking & Full & 400k & 5,000 & \textbf{9.607} & 12.840 \\
\bottomrule
\end{tabular}
\end{table}
