# Supplementary material for: EMG-GPT: Predictive Pretraining on Residual-Quantized EMG Tokens for Hand Pose Estimation
Source: arXiv:2610.05235 source file (2026-10-04)
Supplement: Supplementary file 13 [file tab_appendix_past_only.tex]

\begin{table}[h!]
\centering
\small
\caption{Matched 25-Hz frozen-transfer control for same-target-frame depth conditioning (validation, seed 123). Past-only removes realized coarser target-depth codes.}
\label{tab:appendix-past-only}
\begin{tabular}{@{}lrrrr@{}}
\toprule
GPT step & \multicolumn{2}{c}{Regression MAE ($^\circ$)} & \multicolumn{2}{c}{Tracking MAE ($^\circ$)} \\
\cmidrule(lr){2-3}\cmidrule(l){4-5}
& Standard & Past-only & Standard & Past-only \\
\midrule
160k & 14.366 & 14.270 & 9.850 & 9.824 \\
200k & 14.419 & 14.246 & 9.840 & 9.841 \\
\bottomrule
\end{tabular}
\end{table}
