# Supplementary material for: EMG-GPT: Predictive Pretraining on Residual-Quantized EMG Tokens for Hand Pose Estimation
Source: arXiv:2610.05235 source file (2026-10-04)
Supplement: Supplementary file 15 [file tab_appendix_temporal_grid.tex]

\begin{table}[h!]
\centering
\small
\caption{Temporal-grid stages used in this study. Both predict 200~ms ahead; the stages differ in sampling cadence and experimental role and are not treated as a matched frequency ablation.}
\label{tab:appendix-temporal-grid}
\begin{tabular}{@{}lrrrrl@{}}
\toprule
Stage & Token rate & Patch & Hop & $\Delta$ & Role \\
\midrule
Initial screens & 5 Hz & 200 ms & 200 ms & 1 & Architecture, depth, capacity, objective \\
Long-run development & 25 Hz & 200 ms & 40 ms & 5 & $K=4$ representation trajectory \\
\bottomrule
\end{tabular}
\end{table}
