# Supplementary material for: EMG-GPT: Predictive Pretraining on Residual-Quantized EMG Tokens for Hand Pose Estimation
Source: arXiv:2610.05235 source file (2026-10-04)
Supplement: Supplementary file 16 [file tab_appendix_tracking_downstream.tex]

\begin{table}[h!]
\centering
\small
\caption{Controlled 25-Hz Tracking velocity-loss ablation on validation (seed 123, frozen GPT, 10k-step downstream budget). Only $\lambda_{\mathrm{vel}}$ changes.}
\label{tab:appendix-tracking-downstream}
\begin{tabular}{@{}lrrrrr@{}}
\toprule
$\lambda_{\mathrm{vel}}$ & MAE ($^\circ$) & User+Stage & Landmark & Pred. speed & Target speed \\
\midrule
0 & 9.84 & 13.10 & 13.27 & 18.1 & 66.4 \\
1 & 9.85 & 13.09 & 13.25 & 19.4 & 66.4 \\
4 & 9.83 & 13.12 & 13.25 & 19.4 & 66.4 \\
\bottomrule
\end{tabular}
\end{table}
